# Supplementary material for: COKE: A Cognitive Knowledge Graph for Machine Theory of Mind
Source: arXiv:2305.05390 source file (2024-05-18)
Supplement: Supplementary file 1 [file AppendixH_ESC_HE.tex]

% Please add the following required packages to your document preamble:
% \usepackage{graphicx}
\begin{table}[]
\centering
% \resizebox{\textwidth}{!}{%
\begin{tabular}{llll}
\toprule
vs.                & \multicolumn{3}{l}{ESC Vanilla}        \\
                   & Win             & Tie      & Lose      \\ \hline
\multicolumn{2}{l}{Fluency}          &          &           \\
\multicolumn{2}{l}{Identification} &          &           \\
Comforting         &                 &          &           \\
Suggestion         &                 &          &           \\ \hline
Overall            &                 &          &           \\ \bottomrule
\end{tabular}%
% }
\caption{ Human evaluation results  (ESC+\cokelm vs.).}
\label{tab-esc-humanevaluation}
\end{table}
