# Supplementary material for: COKE: A Cognitive Knowledge Graph for Machine Theory of Mind
Source: arXiv:2305.05390 source file (2024-05-18)
Supplement: Supplementary file 2 [file AppendixJ_checklist.tex]

% Please add the following required packages to your document preamble:
% \usepackage{graphicx}
% \usepackage[table,xcdraw]{xcolor}
% If you use beamer only pass "xcolor=table" option, i.e. \documentclass[xcolor=table]{beamer}
\begin{table}[h]
\centering
\resizebox{\textwidth}{!}{%
\begin{tabular}{ll}
\toprule
1.	For   all authors... &
   \\ \hline
{\color[HTML]{333333} (a) Do   the main claims made   in the abstract and introduction accurately reflect the paper's contributions   and scope?} &
  {\color[HTML]{FF0000} {[}YES{]}} \\
{\color[HTML]{333333} (b) Have you   read the ethics review guidelines and ensured that your paper conforms to them?} &
  {\color[HTML]{FF0000} {[}YES{]}} \\
{\color[HTML]{333333} (c) Did you   discuss any potential negative societal impacts of your work?} &
  {\color[HTML]{FF0000} {[}YES{]}} \\
{\color[HTML]{333333} (d) Did you   describe the limitations of   your work?} &
  {\color[HTML]{FF0000} {[}YES{]}} \\ \hline
{\color[HTML]{333333} 2. If you are including theoretical results...} &
   \\ \hline
{\color[HTML]{333333} (a) Did you   state the full set of assumptions of all theoretical results?} &
  {[}N/A{]} \\
{\color[HTML]{333333} (b) Did you   include complete proofs of   all theoretical results?} &
  {[}N/A{]} \\ \hline
{\color[HTML]{333333} 3.  If you ran   experiments...} &
   \\ \hline
{\color[HTML]{333333} \begin{tabular}[c]{@{}l@{}}(a) Did you include the code, data, and instructions needed   to reproduce the   main experimental results \\      (either in the supplemental material or as a URL)?\end{tabular}} &
  {\color[HTML]{FF0000} {[}YES{]}} \\
{\color[HTML]{333333} (b) Did you   specify all the training details (e.g., data splits, hyperparameters, how they were   chosen)?} &
  {\color[HTML]{FF0000} {[}YES{]}} \\
{\color[HTML]{333333} (c) Did you   report error bars (e.g.,   with respect to the random seed after running experiments multiple   times)?} &
  {\color[HTML]{FF0000} {[}YES{]}} \\
{\color[HTML]{333333} (d) Did you   include the amount of compute and the type of resources used (e.g., type of GPUs, internal cluster, or cloud   provider)? {[}Yes{]}} &
  {\color[HTML]{FF0000} {[}YES{]}} \\ \hline
{\color[HTML]{333333} 4.If you are   using existing assets (e.g., code, data, models) or curating/releasing new   assets...} &
   \\ \hline
{\color[HTML]{333333} (a) If your   work uses existing assets, did you cite the creators?} &
  {\color[HTML]{FF0000} {[}YES{]}} \\
{\color[HTML]{333333} (b) Did you   mention the license of   the assets?} &
  {\color[HTML]{FF0000} {[}YES{]}} \\
{\color[HTML]{333333} (c) Did you   include any new assets either   in the supplemental material or as a URL?} &
  {\color[HTML]{FF0000} {[}YES{]}} \\
{\color[HTML]{333333} (d) Did you   discuss whether and how consent was obtained from people whose data you're   using/curating?} &
  {\color[HTML]{FF0000} {[}YES{]}} \\
{\color[HTML]{333333} (e) Did you discuss whether the data you are using/curating   contains personally identifiable information or offensive content?} &
  {\color[HTML]{FF0000} {[}YES{]}} \\ \hline
{\color[HTML]{333333} 5. If you   used crowdsourcing or conducted research with human subjects...} &
   \\ \hline
{\color[HTML]{333333} (a) Did you   include the full text of instructions given to participants and screenshots,   if applicable?} &
  {\color[HTML]{FF0000} {[}YES{]}} \\
{\color[HTML]{333333} (b) Did you   describe any potential participant risks, with links to Institutional Review Board (IRB) approvals, if   applicable?} &
  {[}N/A{]} \\
{\color[HTML]{333333} (c) Did you include the estimated hourly wage paid to   participants and the total amount spent on participant compensation?} &
  {\color[HTML]{FF0000} {[}YES{]}} \\ \bottomrule
\end{tabular}%
}
\label{tab-checklist}
\end{table}
